# Supplementary material for: Inference of joint conformational distributions from separately-acquired experimental measurements
Source: arXiv:2010.15612 ancillary file (2020-10-29)
Supplement: Supplementary file 1 [file correlation_structure_si.pdf]

# Supplemental Materials: Inference of joint conformational distributions from separately-acquired experimental measurements

Jennifer M. Hays, Emily Boland, Peter M. Kasson  
(Dated: October 13, 2020)

## METHODS

### Alternating-access transporter

To validate the Ensemble Estimation from Separate Measurements (EESM) approach, we performed 500 iterations of the method on the system shown in Fig. 1 and compared the estimated joint distribution with the true distribution. The true distribution was calculated analytically as described below in *Analytical calculation of the alternating-access transporter joint distribution*. Details of EESM simulations for the transporter follow in *EESM estimation of the alternating-access transporter joint distribution*.

#### *Analytical calculation of the alternating-access transporter joint distribution*

We analytically calculated the probability distributions shown in Fig. 2 A-B using the parameters in Table I and the following equations. The probability of observing a particular channel width is given by

$$p(\ell) \propto e^{-\frac{3}{2}(\ell-1)^2} \quad (\text{S1})$$

and the probability of observing a particular distance  $d$  at either mouth of the channel given a particular channel width  $\ell$  is:

$$p(d|\ell) \propto \begin{cases} e^{-\frac{3}{2}(\ell-1)^2} & \ell - 1 \leq d \leq \ell + 1 \\ 0 & \text{otherwise} \end{cases} \quad (\text{S2})$$

To calculate  $p(d)$ , we integrate over the channel widths. The joint probability distribution shown in Fig. 2A is then the convolution of Eq. S2 with itself.

The probability of observing a pair of distances  $(d_1, d_2)$  given a channel width  $\ell$  is:

$$p(d_1, d_2|\ell) = p(d_1|\ell)p(d_2|\ell) \quad (\text{S3})$$

The symmetry constraint determines the probability  $p(d_1|d_2, \ell)$ :

$$p(d_1|d_2, \ell) \propto \begin{cases} 1 & d_1 = d_2 + 2 \sin \theta \\ 0 & \text{otherwise} \end{cases} \quad (\text{S4})$$

From combining equations S1-S4 and marginalizing over the channel widths, we can calculate the joint probability distribution in Fig. 2B.

TABLE I: Parameter choices for toy model. All distance values are unitless, angles are given in radians

| Parameter          | Value     |
|--------------------|-----------|
| $\alpha$           | $3 k_B T$ |
| $\ell_0$           | 1         |
| Length of each rod | 2         |
| $\theta_{\min}$    | $-\pi/6$  |
| $\theta_{\max}$    | $\pi/6$   |

*EESM estimation of the alternating-access transporter joint distribution*

To estimate the toy model’s joint distribution, we iteratively:

1. Select a set of distances  $(d_1, d_2)$  by sampling from the distribution shown in Fig. 2A.
2. Determine the conformation  $c$  associated with  $(d_1, d_2)$  using the constraints.
3. Calculate the work required to drive the conformation of the previous iteration to the conformation of (2).

When the EESM iterations are performed sequentially, the work is a function of the previous iteration’s initial state and the final state:

$$W(x_i \rightarrow x_f) = \frac{1}{2} \alpha (\ell_f - \ell_i)^2$$

If the iterations are performed entirely in parallel and the initial conformation is drawn from equilibrium, then the work is simply

$$W(x_i \rightarrow x_f) = \frac{1}{2} \alpha (\ell_f - \ell_0)^2$$

After obtaining work estimates using this resampling procedure, we calculate the free energy as a function of the distance variables  $D_1, D_2$  using the Jarzynski equality. To obtain the free energy  $\Delta G(\{x\} | D_1 = d_1, D_2 = d_2)$ , we average the exponential work values over all trials where  $x_f$  has  $D_1 = d_1, D_2 = d_2$ :

$$e^{-\beta \Delta G(\{x\} | d_1, d_2)} = \langle e^{-\beta W(x_i \rightarrow x_f | d_1, d_2)} \rangle$$

After approximately 500 iterations, both the sequential and parallel procedures converge on the analytically determined joint distribution (Fig. 3).

**Estimating the joint distribution of separately-acquired DEER measurements on syntaxin**

Because of the complexity inherent in a flexible protein of syntaxin’s size, we cannot calculate the joint distribution of pairwise distance distributions analytically. We therefore estimated the free energy difference between a syntaxin reference ensemble,  $\{X'\}$ , and a final conformational estimate,  $\{X\}$ , by calculating the non-equilibrium work done on syntaxin over multiple MD pulling experiments each restrained to a random sample from the DEER-derived pairwise distance distributions. The Jarzynski equality (Eq. 3) specifies how these non-equilibrium work measurements yield the free energy difference (and thus relative probability) between the reference ensemble and each final ensemble member, specified by its target distance tuple  $(d_1, d_2, d_3)$ . Details of the reference ensemble, pulling experiments, and final conformational estimate follow.

*Selection of the reference ensemble*

We used as a reference ensemble a set of conformations generated using a maximum-entropy refinement method assuming that the experimental DEER measurements were uncorrelated (Fig S1A). This reference ensemble and the refinement method used to obtain it have been previously published[S1]. Approximately 250 syntaxin structures were sampled from this ensemble.

*Molecular dynamics pulling experiments*

To sample the free energy landscape, we ran a total of  $1.3\mu\text{s}$  of MD simulation using the EESM protocol. Simulations were performed using an all-atom representation of syntaxin in explicit solvent, with approximately 90,000 TIP3P water molecules, 150 mM NaCl, and no net charge. Simulations were run in Gromacs[S2], using the CHARMM36 force field[S3]. The system was run under NPT conditions using the velocity-rescaling thermostat[S4] at 310K with a 2 ps time constant and pressure maintained at 1 bar using the Parrinello-Rahman barostat[S5] with a 10-ps time

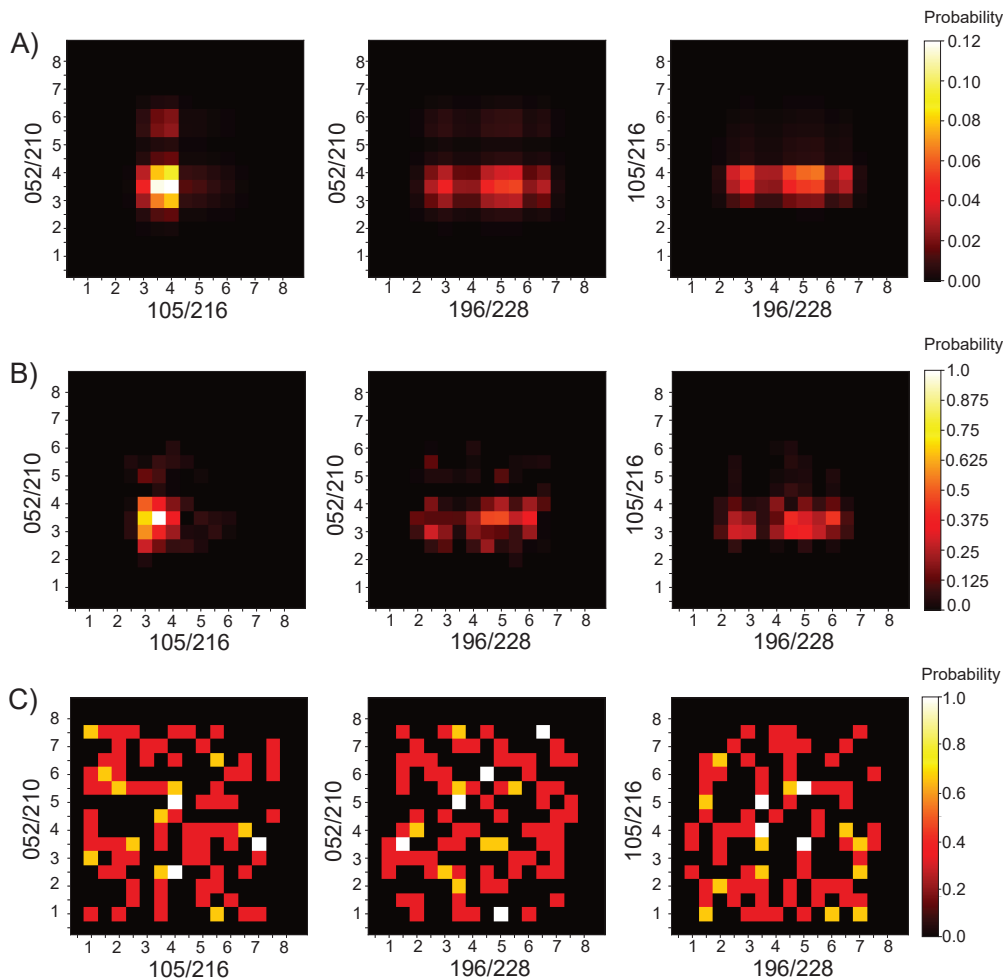

FIG. S1: **2D projections showing uncorrelated DEER distributions, starting structures, and target coordinates for MD pulling simulations.** Plotted in (A) are the 2D convolutions of each pair of DEER distributions used to generate the reference ensemble  $\{X'\}$ . Plotted in (B) are corresponding 2D distributions for the distance variables corresponding to Starting structures for each pulling simulation. These structures were sampled with replacement from the reference ensemble and, as expected, their distribution is similar to the uncorrelated distributions in (A). Finally, the target tuples  $(d_1, d_2, d_3)$  are plotted in (C), which approximate a uniform distribution over the space.

constant. Covalent bonds were constrained using LINCS, and long-range electrostatics were treated using Particle Mesh Ewald[S6].

We consider the free-energy landscape of syntaxin using the experimental observables (the distances measured via DEER) as order parameters. Let us denote these three distance variables by the tuple  $(D_1, D_2, D_3)$ . We estimated the free-energy landscape by selecting 100 tuples in this space,  $(d_1, d_2, d_3)$ , by randomly sampling from a uniform distribution over the three distance variables (Fig. S1C). We then ran ten biased MD simulations per target tuple: we randomly sampled ten structures  $\{x'\}$  from the reference ensemble  $\{X'\}$  (Fig. S1B) and drove the distance variable  $D_i$  to the target  $d_i$ . The maximum-entropy biasing potential we use was originally formulated in [S7], and details of our implementation can be found in [S1].

Due to the ruggedness of the free-energy landscape, pulling runs from some starting conformations  $x'$  did not converge to their target tuples. Simulations were run for a maximum of 100 ns; runs with any distance variable  $D_i$  that did not converge to within  $1\text{\AA}$  of the target  $d_i$  were marked as unconverged, with an upper limit of infinite work required to converge to  $d_i$ . Work calculations and Jarzynski estimates are described in the following section.

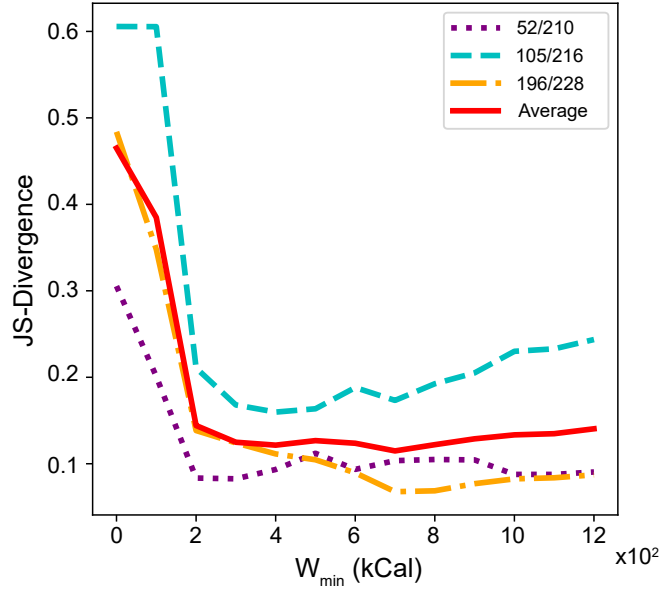

FIG. S2: **Thresholding mitigates the effect of small, outlier work values.** The exponentially weighted terms in the Jarzynski equality imbue extreme sensitivity to outliers, in this case anomalously low work values. This is solved by adding a thresholding term  $W_i = \max(W_i, W_{\min})$ , as described in the text. Average disagreement between DEER-derived distributions and the EESM distributions (red), quantified as JS divergence, decreases rapidly as  $W_{\min}$  increases from 0 to 200 kcal before reaching a plateau. Average disagreement continues to decrease until it reaches a local minimum at  $W_{\min} = 400$  kcal. Although a global minimum occurs at  $W_{\min} = 700$  kcal, we selected  $W_{\min} = 400$  kcal because it likely introduces a smaller perturbation to the system. Indeed, the local minima of the individual distributions occur more often near  $W_{\min} = 400$  kcal relative to  $W_{\min} = 700$  kcal.

#### Final ensemble estimation

We estimated the work required to bias a distance variable  $D_i$  to its target  $d_i$ , for each converged run, as the numerical integral  $\int F dx$ . The maximum entropy restraint we apply utilizes a constant force, so the integral reduces to  $F \sum_t [d_i(t) - d_i(t-1)]$  where  $d_i(t)$  is the current distance value. We performed this calculation for all three distributions described by the target tuple  $(d_1, d_2, d_3)$ , and then summed them together to obtain the total work value for a single run. This process was repeated for all runs.

An estimate of the free energy difference from the reference ensemble was then calculated using the set of work values associated with each target distance tuple  $(d_1, d_2, d_3)$ . As discussed above, unconverged runs were assigned an infinite work value with associated probability of zero. The resulting free energy estimates and associated probabilities were then normalized across distance samples to obtain a final EESM ensemble estimate.

As our simulations are run with finite sampling, we expect there to be some outlier work values. In this case, because the Jarzynski equality involves averaging of *exponentially* weighted work values, low-valued outliers can dominate the calculation. We therefore applied a thresholding correction to mitigate the effects of these outliers: we set all work values  $W$  to  $\max(W, W_{\min})$ , where  $W_{\min}$  is a constant we set based on the ensemble agreement with experimental data. To select a  $W_{\min}$ , we tested values from 0-1200 in increments of 100. We then compared the degree of disagreement between the estimation obtained with this threshold value and the experimental data for each measured distribution, as well as the average level of disagreement, as quantified by Jensen-Shannon Divergence (Fig. S2).

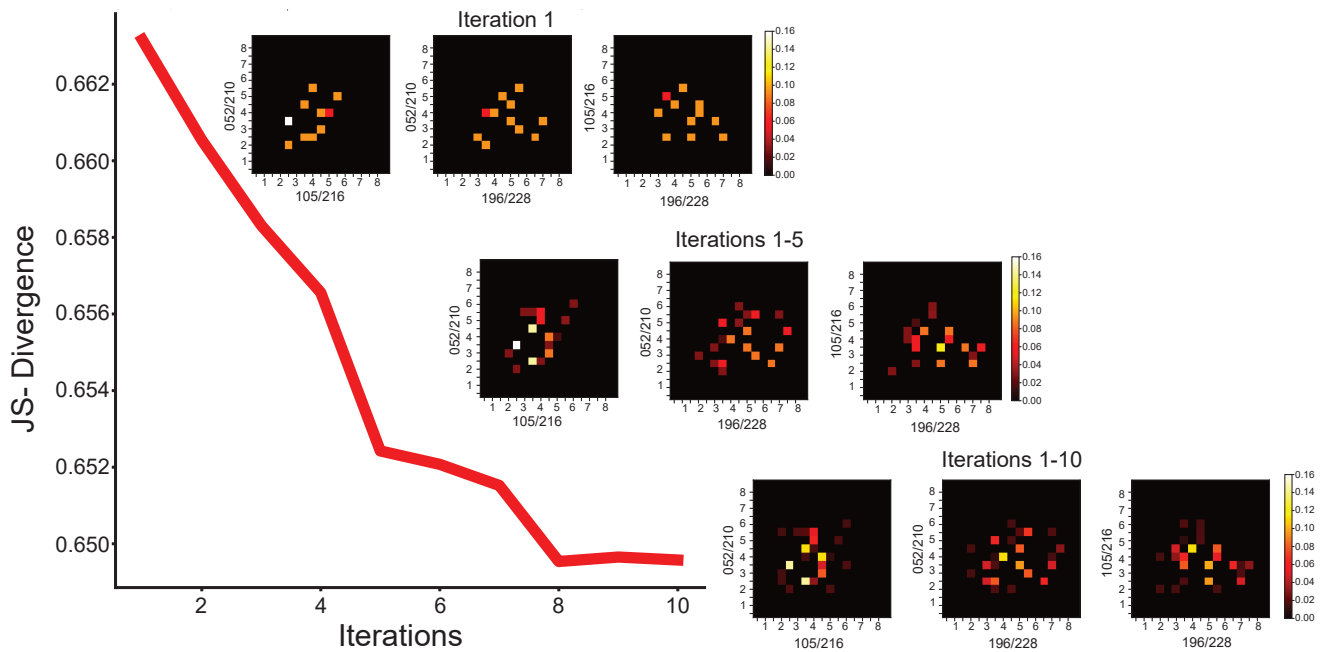

FIG. S3: **Evolution of the EESM joint distribution compared to the convolution of experimental distributions:** Plotted on the left is the disagreement between the DEER-derived convolved distribution and the EESM distribution, quantified as Jensen-Shannon (JS) divergence. This quantity decreases monotonically throughout the first eight cumulative iterations, then stabilizes at a non-zero value, demonstrating that EESM method produces a joint distribution that is different than experimental convolution. The small numerical change in JS divergence (from 0.663 to 0.649) reflects a substantial change in the estimated joint distribution. Projections of the joint distribution are shown on the right after 1, 5, and 10 iterations.

## REFERENCES

- 
- [S1] J. M. Hays, D. S. Cafiso, and P. M. Kasson, *J. Phys. Chem. Lett.* pp. 3410–3414 (2019), ISSN 1948-7185.
  - [S2] S. Pronk, S. Páll, R. Schulz, P. Larsson, P. Bjelkmar, R. Apostolov, M. R. Shirts, J. C. Smith, P. M. Kasson, D. van der Spoel, et al., *Bioinformatics* **29**, 845 (2013), ISSN 1367-4811.
  - [S3] J. Huang and A. D. MacKerell, *J Comput Chem* **34** (2013), ISSN 0192-8651.
  - [S4] G. Bussi, D. Donadio, and M. Parrinello, *The Journal of Chemical Physics* **126**, 014101 (2007), ISSN 0021-9606.
  - [S5] M. Parrinello and A. Rahman, *J. Chem. Phys.* **76**, 2662 (1982), ISSN 0021-9606.
  - [S6] T. Darden, D. York, and L. Pedersen, **98**, 10089 (1993).
  - [S7] A. D. White and G. A. Voth, *Journal of chemical theory and computation* **10**, 3023 (2014).
  - [S8] D. Dawidowski and D. S. Cafiso, *Biophys. J.* **104**, 1585 (2013), ISSN 00063495.

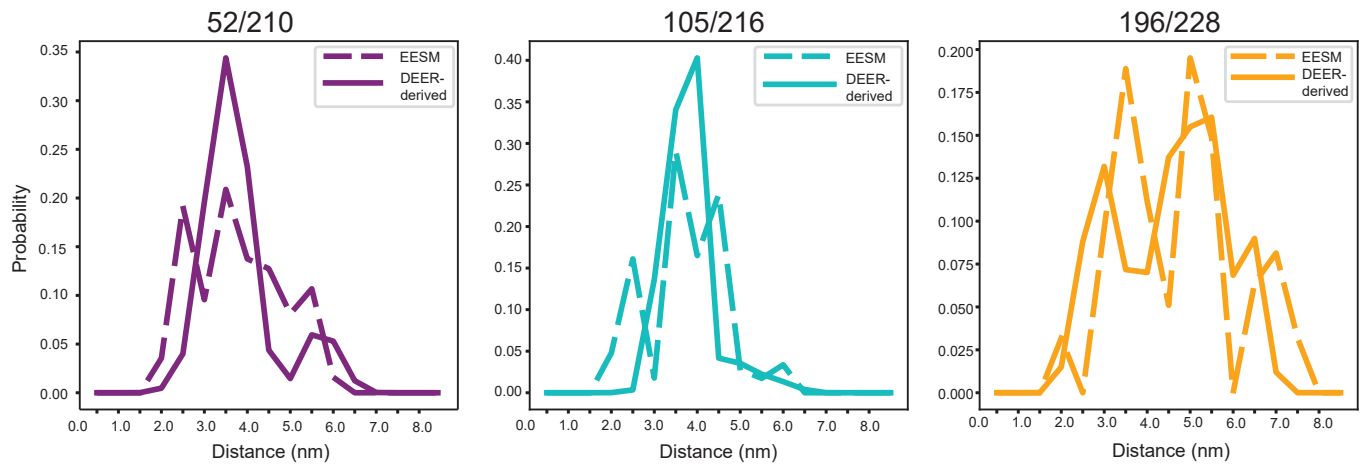

FIG. S4: **The one-dimensional projections of the EESM joint distribution approximate the experimental distributions.** The EESM projections share the same major peaks as and sample the full width of the DEER-derived distributions. The EESM distributions are less sharply peaked than their DEER equivalents, but this is largely because the form of the biasing potential in our simulations is deliberately chosen so as to minimally perturb the MD Hamiltonian[S1]. This often results in higher entropy simulation distributions.

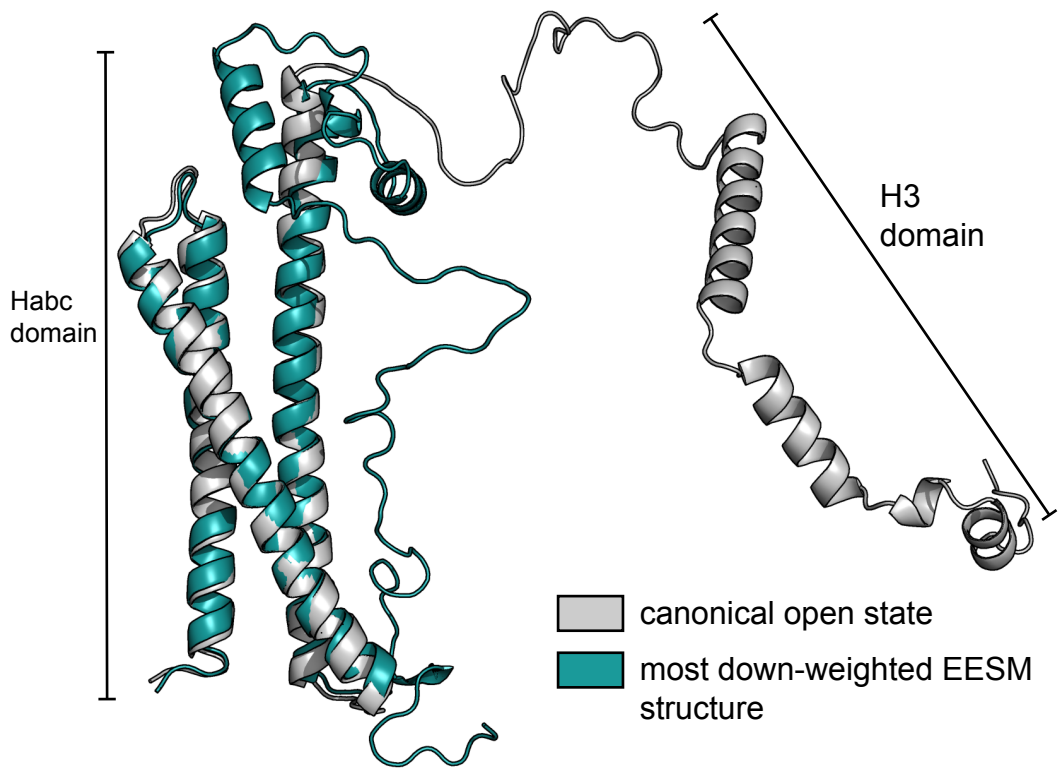

FIG. S5: **EESM down-weights open-state structures that are unlikely relative to the hypothesized open state.** Although no experimentally-determined open-state structure of syntaxin exists, it is generally thought that the H3 domain dissociates completely from the Habc domain to form the hypothesized structure generated by Dawidowski and Cafiso[S8] and rendered in grey. In contrast, the teal structure retains some but not all of the contacts between H3 and Habc, which is likely energetically unfavorable. This teal structure is allowed by the convolution of the experimental distributions, but the EESM method correctly identifies it as high-free-energy and maximally down-weights it. The teal structure is the same as the structure rendered in Fig. 4.
